# Supplementary material for: On the generalizability of machine-learning-assisted anisotropy mappings for predictive turbulence modelling
Source: arXiv:2206.05226 ancillary file (2022-08-11)
Supplement: Supplementary file 1 [file IJCFD_supplemental_material.pdf]

# On the generalizability of machine-learning-assisted anisotropy mappings for predictive turbulence modelling

## Supplemental material

Ryley McConkey, Eugene Yee, Fue-Sang Lien

August 2022

This material contains extra generalizability tests that could not be included in the original manuscript due to space. While the original manuscript includes the generalizability test of the XGBoost model on a few selected flows, all tests for all models and all training datasets are presented here.

For each training set and for each model type, a hyperparameter optimization procedure was completed (see the original paper for more details). Then, these optimized models were tested on the hold-out test flows. This material is organized by test case. For a given test case, optimized models on various training sets are compared.

In total, there are 60 generalizability tests consisting of 3 model types  $\times$  4 training sets  $\times$  5 test cases. All test cases were held out of all training sets (see Table 3 in the paper). Each generalizability test is represented by a figure in this supplementary material showing the true and predicted values of the tensor basis coefficients  $g^{(1)}$ ,  $g^{(2)}$ , and  $g^{(3)}$ .

## Contents

|          |                                 |          |
|----------|---------------------------------|----------|
| <b>1</b> | <b>Periodic hills test set</b>  | <b>3</b> |
| 1.1      | PHLL4 training set . . . . .    | 3        |
| 1.1.1    | Neural network . . . . .        | 3        |
| 1.1.2    | Random forest . . . . .         | 3        |
| 1.1.3    | XGBoost . . . . .               | 4        |
| 1.2      | BUMP4 training set . . . . .    | 4        |
| 1.2.1    | Neural network . . . . .        | 4        |
| 1.2.2    | Random forest . . . . .         | 4        |
| 1.2.3    | XGBoost . . . . .               | 5        |
| 1.3      | DUCT15 training set . . . . .   | 5        |
| 1.3.1    | Neural network . . . . .        | 5        |
| 1.3.2    | Random forest . . . . .         | 5        |
| 1.3.3    | XGBoost . . . . .               | 6        |
| 1.4      | FULL training set . . . . .     | 6        |
| 1.4.1    | Neural network . . . . .        | 6        |
| 1.4.2    | Random forest . . . . .         | 6        |
| 1.4.3    | XGBoost . . . . .               | 7        |
| <b>2</b> | <b>Parametric bump test set</b> | <b>7</b> |
| 2.1      | PHLL4 training set . . . . .    | 7        |
| 2.1.1    | Neural network . . . . .        | 7        |
| 2.1.2    | Random forest . . . . .         | 8        |
| 2.1.3    | XGBoost . . . . .               | 8        |
| 2.2      | BUMP4 training set . . . . .    | 8        |
| 2.2.1    | Neural network . . . . .        | 8        |
| 2.2.2    | Random forest . . . . .         | 9        |
| 2.2.3    | XGBoost . . . . .               | 9        |
| 2.3      | DUCT15 training set . . . . .   | 9        |
| 2.3.1    | Neural network . . . . .        | 9        |
| 2.3.2    | Random forest . . . . .         | 10       |
| 2.3.3    | XGBoost . . . . .               | 10       |
| 2.4      | FULL training set . . . . .     | 10       |
| 2.4.1    | Neural network . . . . .        | 10       |

|          |                                              |           |
|----------|----------------------------------------------|-----------|
| 2.4.2    | Random forest                                | 11        |
| 2.4.3    | XGBoost                                      | 11        |
| <b>3</b> | <b>Square duct test set</b>                  | <b>12</b> |
| 3.1      | PHLL4 training set                           | 12        |
| 3.1.1    | Neural network                               | 12        |
| 3.1.2    | Random forest                                | 12        |
| 3.1.3    | XGBoost                                      | 13        |
| 3.2      | BUMP4 training set                           | 13        |
| 3.2.1    | Neural network                               | 13        |
| 3.2.2    | Random forest                                | 14        |
| 3.2.3    | XGBoost                                      | 14        |
| 3.3      | DUCT15 training set                          | 15        |
| 3.3.1    | Neural network                               | 15        |
| 3.3.2    | Random forest                                | 15        |
| 3.3.3    | XGBoost                                      | 16        |
| 3.4      | FULL training set                            | 16        |
| 3.4.1    | Neural network                               | 16        |
| 3.4.2    | Random forest                                | 17        |
| 3.4.3    | XGBoost                                      | 17        |
| <b>4</b> | <b>Converging-diverging channel test set</b> | <b>18</b> |
| 4.1      | PHLL4 training set                           | 18        |
| 4.1.1    | Neural network                               | 18        |
| 4.1.2    | Random forest                                | 18        |
| 4.1.3    | XGBoost                                      | 19        |
| 4.2      | BUMP4 training set                           | 19        |
| 4.2.1    | Neural network                               | 19        |
| 4.2.2    | Random forest                                | 20        |
| 4.2.3    | XGBoost                                      | 20        |
| 4.3      | DUCT15 training set                          | 21        |
| 4.3.1    | Neural network                               | 21        |
| 4.3.2    | Random forest                                | 21        |
| 4.3.3    | XGBoost                                      | 22        |
| 4.4      | FULL training set                            | 22        |
| 4.4.1    | Neural network                               | 22        |
| 4.4.2    | Random forest                                | 23        |
| 4.4.3    | XGBoost                                      | 23        |
| <b>5</b> | <b>Curved backward-facing step test set</b>  | <b>24</b> |
| 5.1      | PHLL4 training set                           | 24        |
| 5.1.1    | Neural network                               | 24        |
| 5.1.2    | Random forest                                | 24        |
| 5.1.3    | XGBoost                                      | 25        |
| 5.2      | BUMP4 training set                           | 25        |
| 5.2.1    | Neural network                               | 25        |
| 5.2.2    | Random forest                                | 26        |
| 5.2.3    | XGBoost                                      | 26        |
| 5.3      | DUCT15 training set                          | 27        |
| 5.3.1    | Neural network                               | 27        |
| 5.3.2    | Random forest                                | 27        |
| 5.3.3    | XGBoost                                      | 28        |
| 5.4      | FULL training set                            | 28        |
| 5.4.1    | Neural network                               | 28        |
| 5.4.2    | Random forest                                | 29        |
| 5.4.3    | XGBoost                                      | 29        |

# 1 Periodic hills test set

## 1.1 PHLL4 training set

### 1.1.1 Neural network

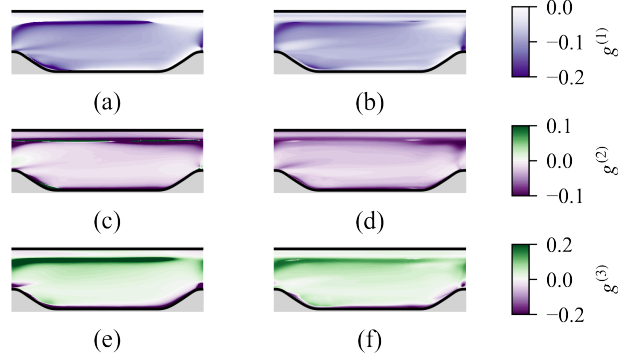

Figure 1: Generalizability test on the periodic hills test case for the neural network model. Here, the training dataset is the periodic hills PHLL4 set: (a) true  $g^{(1)}$  field; (b) predicted  $g^{(1)}$  field; (c) true  $g^{(2)}$  field; (d) predicted  $g^{(2)}$  field; (e) true  $g^{(3)}$  field; and, (f) predicted  $g^{(3)}$  field.

### 1.1.2 Random forest

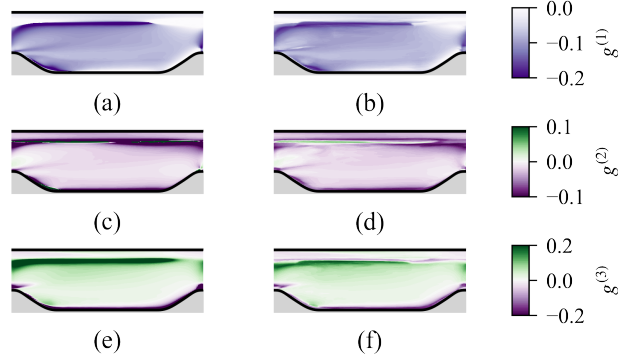

Figure 2: Generalizability test on the periodic hills test case for the random forest model. Here, the training dataset is the periodic hills PHLL4 set: (a) true  $g^{(1)}$  field; (b) predicted  $g^{(1)}$  field; (c) true  $g^{(2)}$  field; (d) predicted  $g^{(2)}$  field; (e) true  $g^{(3)}$  field; and, (f) predicted  $g^{(3)}$  field.

### 1.1.3 XGBoost

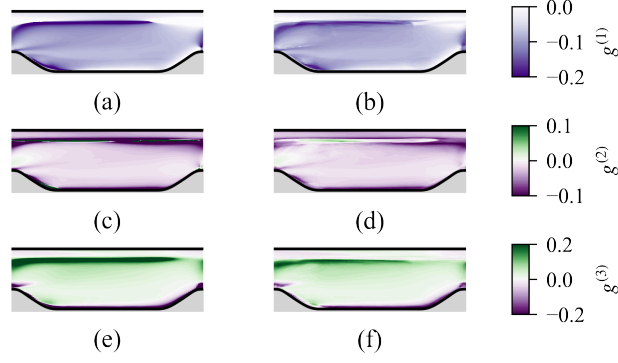

Figure 3: Generalizability test on the periodic hills test case for the XGBoost model. Here, the training dataset is the periodic hills PHLL4 set: (a) true  $g^{(1)}$  field; (b) predicted  $g^{(1)}$  field; (c) true  $g^{(2)}$  field; (d) predicted  $g^{(2)}$  field; (e) true  $g^{(3)}$  field; and, (f) predicted  $g^{(3)}$  field.

## 1.2 BUMP4 training set

### 1.2.1 Neural network

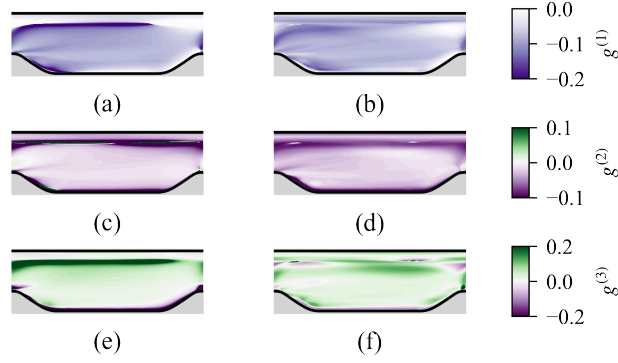

Figure 4: Generalizability test on the periodic hills test case for the neural network model. Here, the training dataset is the parametric bump BUMP4 set: (a) true  $g^{(1)}$  field; (b) predicted  $g^{(1)}$  field; (c) true  $g^{(2)}$  field; (d) predicted  $g^{(2)}$  field; (e) true  $g^{(3)}$  field; and, (f) predicted  $g^{(3)}$  field.

### 1.2.2 Random forest

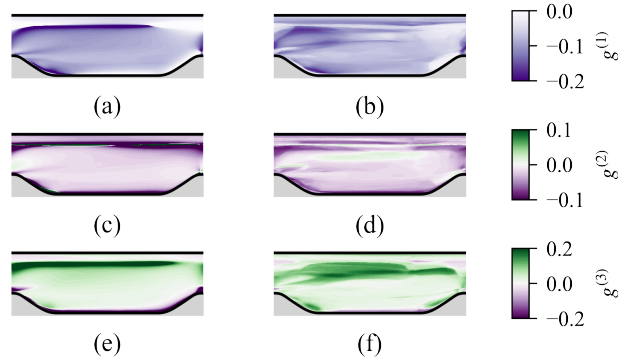

Figure 5: Generalizability test on the periodic hills test case for the random forest model. Here, the training dataset is the parametric bump BUMP4 set: (a) true  $g^{(1)}$  field; (b) predicted  $g^{(1)}$  field; (c) true  $g^{(2)}$  field; (d) predicted  $g^{(2)}$  field; (e) true  $g^{(3)}$  field; and, (f) predicted  $g^{(3)}$  field.

### 1.2.3 XGBoost

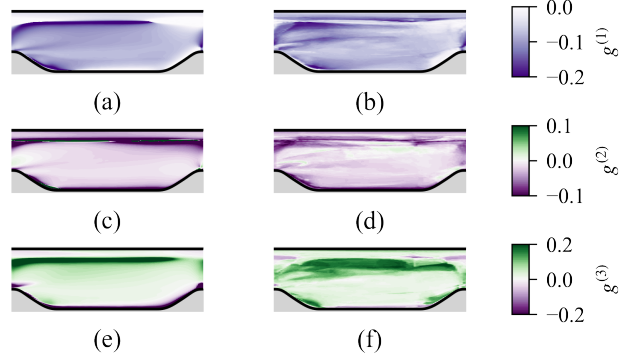

Figure 6: Generalizability test on the periodic hills test case for the XGBoost model. Here, the training dataset is the parametric bump BUMP4 set: (a) true  $g^{(1)}$  field; (b) predicted  $g^{(1)}$  field; (c) true  $g^{(2)}$  field; (d) predicted  $g^{(2)}$  field; (e) true  $g^{(3)}$  field; and, (f) predicted  $g^{(3)}$  field.

## 1.3 DUCT15 training set

### 1.3.1 Neural network

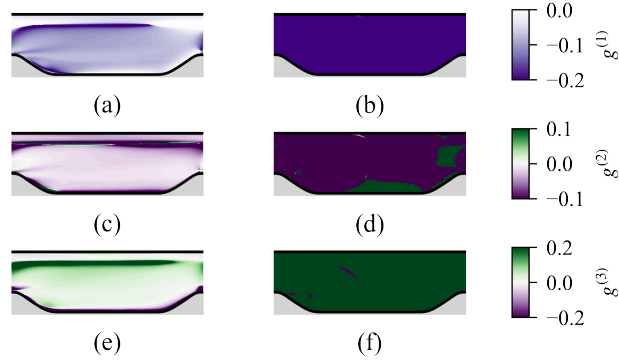

Figure 7: Generalizability test on the periodic hills test case for the neural network model. Here, the training dataset is the square duct DUCT15 set: (a) true  $g^{(1)}$  field; (b) predicted  $g^{(1)}$  field; (c) true  $g^{(2)}$  field; (d) predicted  $g^{(2)}$  field; (e) true  $g^{(3)}$  field; and, (f) predicted  $g^{(3)}$  field.

### 1.3.2 Random forest

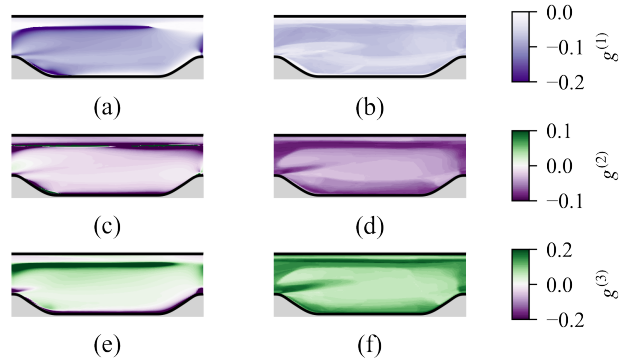

Figure 8: Generalizability test on the periodic hills test case for the random forest model. Here, the training dataset is the square duct DUCT15 set: (a) true  $g^{(1)}$  field; (b) predicted  $g^{(1)}$  field; (c) true  $g^{(2)}$  field; (d) predicted  $g^{(2)}$  field; (e) true  $g^{(3)}$  field; and, (f) predicted  $g^{(3)}$  field.

### 1.3.3 XGBoost

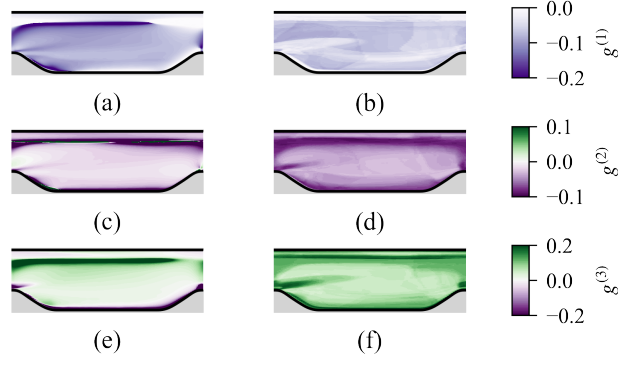

Figure 9: Generalizability test on the periodic hills test case for the XGBoost model. Here, the training dataset is the square duct DUCT15 set: (a) true  $g^{(1)}$  field; (b) predicted  $g^{(1)}$  field; (c) true  $g^{(2)}$  field; (d) predicted  $g^{(2)}$  field; (e) true  $g^{(3)}$  field; and, (f) predicted  $g^{(3)}$  field.

## 1.4 FULL training set

### 1.4.1 Neural network

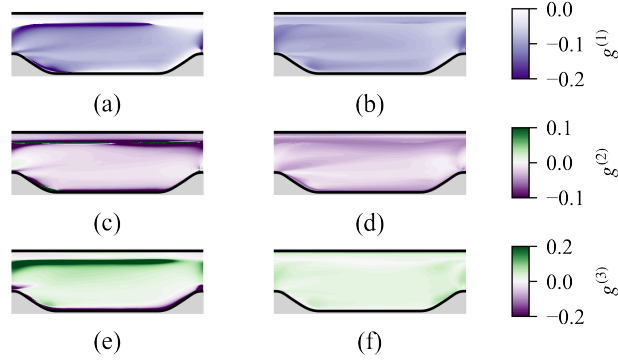

Figure 10: Generalizability test on the periodic hills test case for the neural network model. Here, the training dataset is the FULL set: (a) true  $g^{(1)}$  field; (b) predicted  $g^{(1)}$  field; (c) true  $g^{(2)}$  field; (d) predicted  $g^{(2)}$  field; (e) true  $g^{(3)}$  field; and, (f) predicted  $g^{(3)}$  field.

### 1.4.2 Random forest

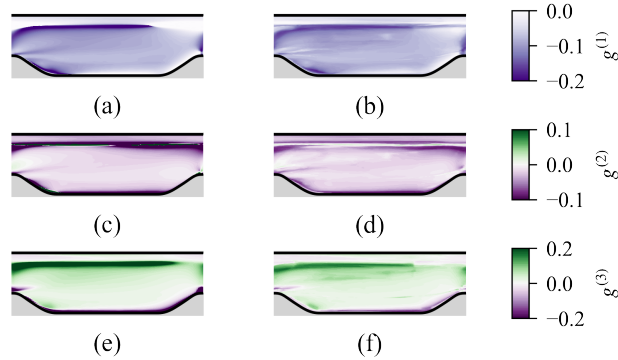

Figure 11: Generalizability test on the periodic hills test case for the random forest model. Here, the training dataset is the FULL set: (a) true  $g^{(1)}$  field; (b) predicted  $g^{(1)}$  field; (c) true  $g^{(2)}$  field; (d) predicted  $g^{(2)}$  field; (e) true  $g^{(3)}$  field; and, (f) predicted  $g^{(3)}$  field.

### 1.4.3 XGBoost

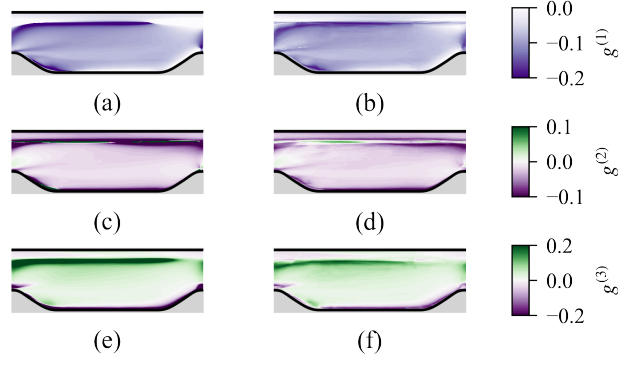

Figure 12: Generalizability test on the periodic hills test case for the XGBoost model. Here, the training dataset is the FULL set: (a) true  $g^{(1)}$  field; (b) predicted  $g^{(1)}$  field; (c) true  $g^{(2)}$  field; (d) predicted  $g^{(2)}$  field; (e) true  $g^{(3)}$  field; and, (f) predicted  $g^{(3)}$  field.

## 2 Parametric bump test set

### 2.1 PHLL4 training set

#### 2.1.1 Neural network

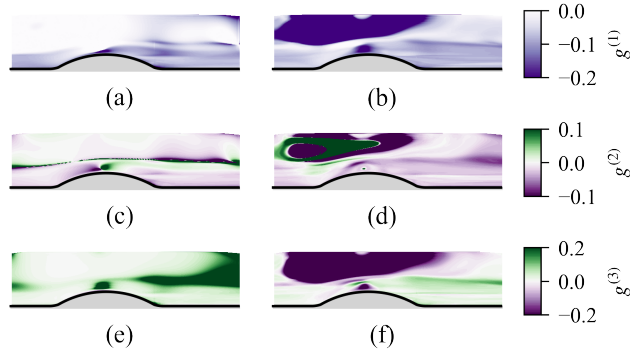

Figure 13: Generalizability test on the parametric bumps test case for the neural network model. Here, the training dataset is the periodic hills PHLL4 set: (a) true  $g^{(1)}$  field; (b) predicted  $g^{(1)}$  field; (c) true  $g^{(2)}$  field; (d) predicted  $g^{(2)}$  field; (e) true  $g^{(3)}$  field; and, (f) predicted  $g^{(3)}$  field.

### 2.1.2 Random forest

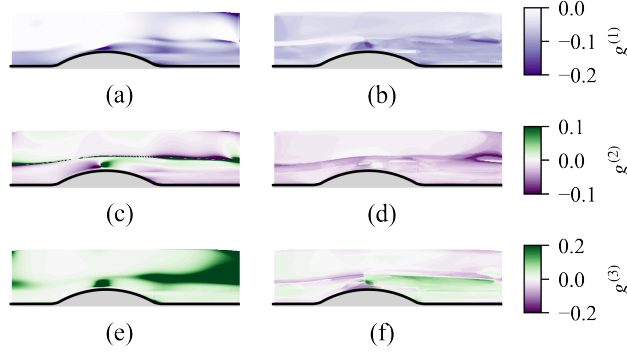

Figure 14: Generalizability test on the parametric bumps test case for the random forest model. Here, the training dataset is the periodic hills PHLL4 set: (a) true  $g^{(1)}$  field; (b) predicted  $g^{(1)}$  field; (c) true  $g^{(2)}$  field; (d) predicted  $g^{(2)}$  field; (e) true  $g^{(3)}$  field; and, (f) predicted  $g^{(3)}$  field.

### 2.1.3 XGBoost

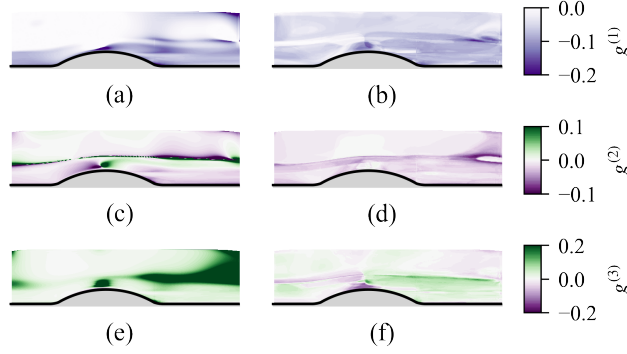

Figure 15: Generalizability test on the parametric bumps test case for the XGBoost model. Here, the training dataset is the periodic hills PHLL4 set: (a) true  $g^{(1)}$  field; (b) predicted  $g^{(1)}$  field; (c) true  $g^{(2)}$  field; (d) predicted  $g^{(2)}$  field; (e) true  $g^{(3)}$  field; and, (f) predicted  $g^{(3)}$  field.

## 2.2 BUMP4 training set

### 2.2.1 Neural network

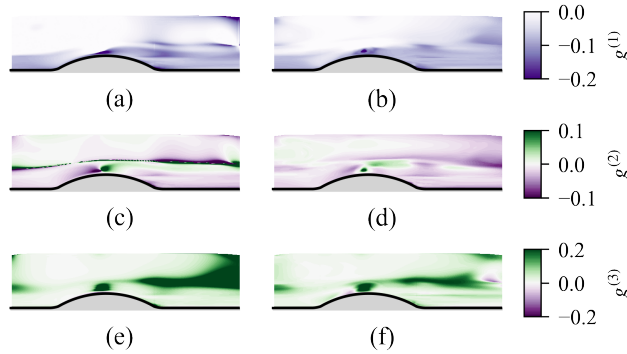

Figure 16: Generalizability test on the parametric bumps test case for the neural network model. Here, the training dataset is the parametric bump BUMP4 set: (a) true  $g^{(1)}$  field; (b) predicted  $g^{(1)}$  field; (c) true  $g^{(2)}$  field; (d) predicted  $g^{(2)}$  field; (e) true  $g^{(3)}$  field; and, (f) predicted  $g^{(3)}$  field.



### 2.2.2 Random forest

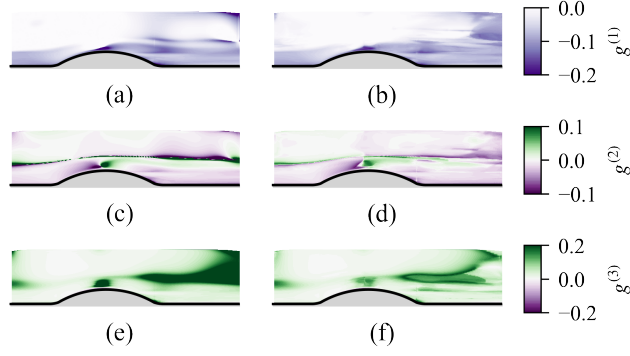

Figure 17: Generalizability test on the parametric bumps test case for the random forest model. Here, the training dataset is the parametric bump BUMP4 set: (a) true  $g^{(1)}$  field; (b) predicted  $g^{(1)}$  field; (c) true  $g^{(2)}$  field; (d) predicted  $g^{(2)}$  field; (e) true  $g^{(3)}$  field; and, (f) predicted  $g^{(3)}$  field.

### 2.2.3 XGBoost

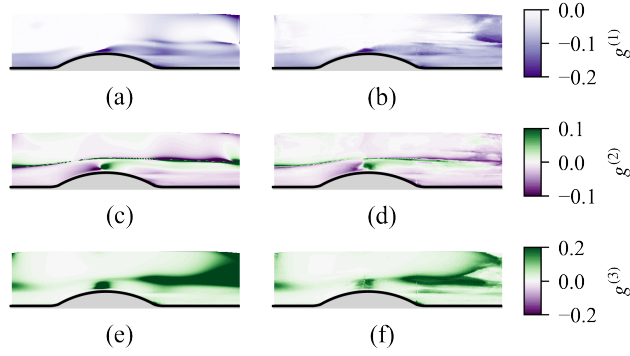

Figure 18: Generalizability test on the parametric bumps test case for the XGBoost model. Here, the training dataset is the parametric bump BUMP4 set: (a) true  $g^{(1)}$  field; (b) predicted  $g^{(1)}$  field; (c) true  $g^{(2)}$  field; (d) predicted  $g^{(2)}$  field; (e) true  $g^{(3)}$  field; and, (f) predicted  $g^{(3)}$  field.

## 2.3 DUCT15 training set

### 2.3.1 Neural network

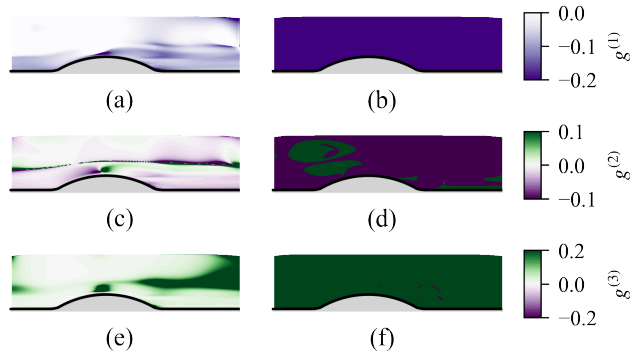

Figure 19: Generalizability test on the parametric bumps test case for the neural network model. Here, the training dataset is the square duct DUCT15 set: (a) true  $g^{(1)}$  field; (b) predicted  $g^{(1)}$  field; (c) true  $g^{(2)}$  field; (d) predicted  $g^{(2)}$  field; (e) true  $g^{(3)}$  field; and, (f) predicted  $g^{(3)}$  field.

### 2.3.2 Random forest

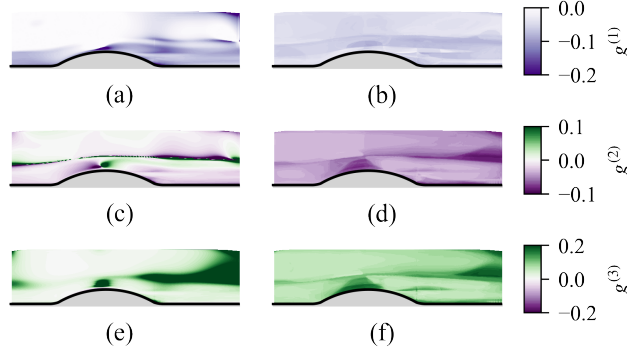

Figure 20: Generalizability test on the parametric bumps test case for the random forest model. Here, the training dataset is the square duct DUCT15 set: (a) true  $g^{(1)}$  field; (b) predicted  $g^{(1)}$  field; (c) true  $g^{(2)}$  field; (d) predicted  $g^{(2)}$  field; (e) true  $g^{(3)}$  field; and, (f) predicted  $g^{(3)}$  field.

### 2.3.3 XGBoost

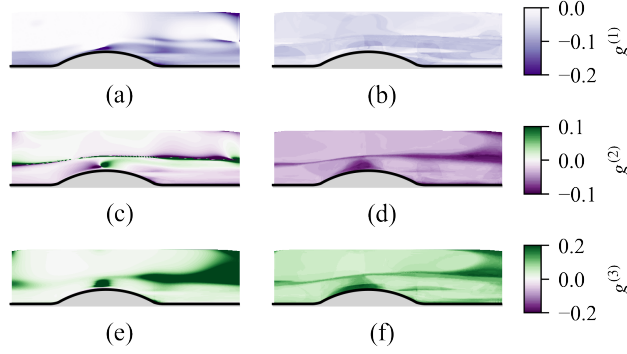

Figure 21: Generalizability test on the parametric bumps test case for the XGBoost model. Here, the training dataset is the square duct DUCT15 set: (a) true  $g^{(1)}$  field; (b) predicted  $g^{(1)}$  field; (c) true  $g^{(2)}$  field; (d) predicted  $g^{(2)}$  field; (e) true  $g^{(3)}$  field; and, (f) predicted  $g^{(3)}$  field.

## 2.4 FULL training set

### 2.4.1 Neural network

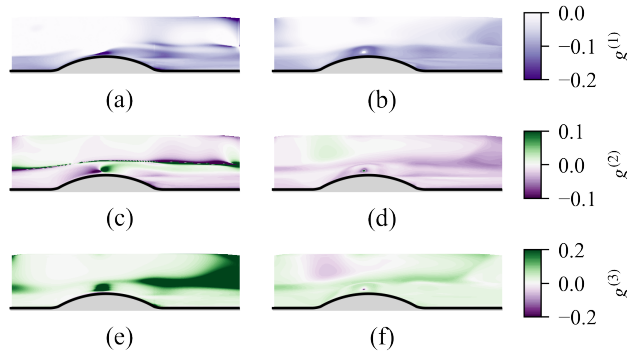

Figure 22: Generalizability test on the parametric bumps test case for the neural network model. Here, the training dataset is the FULL set: (a) true  $g^{(1)}$  field; (b) predicted  $g^{(1)}$  field; (c) true  $g^{(2)}$  field; (d) predicted  $g^{(2)}$  field; (e) true  $g^{(3)}$  field; and, (f) predicted  $g^{(3)}$  field.

### 2.4.2 Random forest

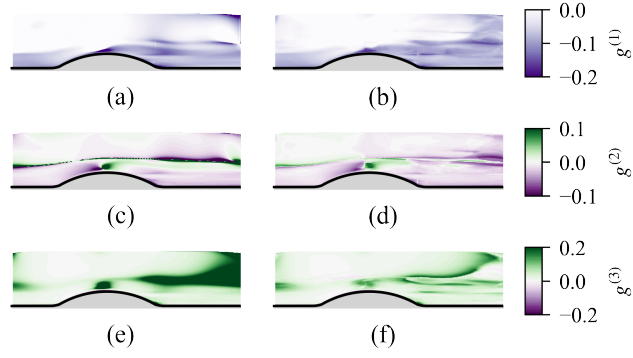

Figure 23: Generalizability test on the parametric bumps test case for the random forest model. Here, the training dataset is the FULL set: (a) true  $g^{(1)}$  field; (b) predicted  $g^{(1)}$  field; (c) true  $g^{(2)}$  field; (d) predicted  $g^{(2)}$  field; (e) true  $g^{(3)}$  field; and, (f) predicted  $g^{(3)}$  field.

### 2.4.3 XGBoost

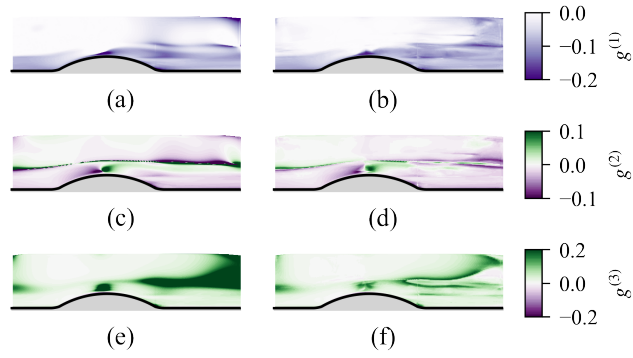

Figure 24: Generalizability test on the parametric bumps test case for the XGBoost model. Here, the training dataset is the FULL set: (a) true  $g^{(1)}$  field; (b) predicted  $g^{(1)}$  field; (c) true  $g^{(2)}$  field; (d) predicted  $g^{(2)}$  field; (e) true  $g^{(3)}$  field; and, (f) predicted  $g^{(3)}$  field.

### 3 Square duct test set

#### 3.1 PHLL4 training set

##### 3.1.1 Neural network

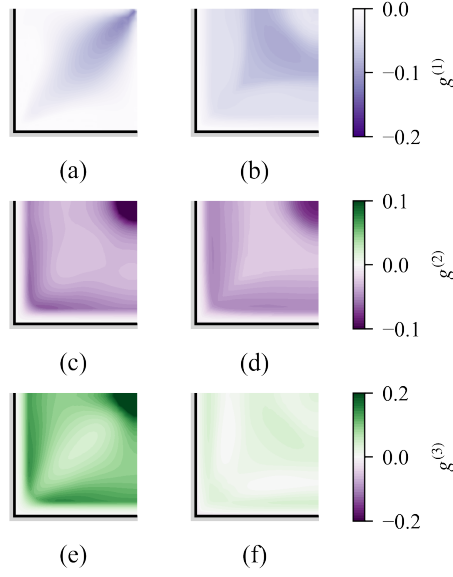

Figure 25: Generalizability test on the square duct test case for the neural network model. Here, the training dataset is the periodic hills PHLL4 set: (a) true  $g^{(1)}$  field; (b) predicted  $g^{(1)}$  field; (c) true  $g^{(2)}$  field; (d) predicted  $g^{(2)}$  field; (e) true  $g^{(3)}$  field; and, (f) predicted  $g^{(3)}$  field.

##### 3.1.2 Random forest

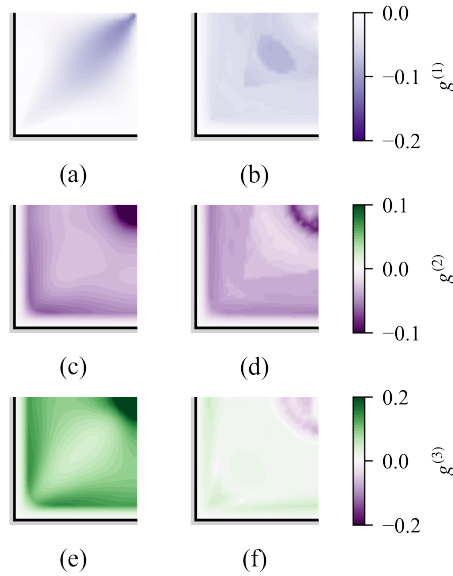

Figure 26: Generalizability test on the square duct test case for the random forest model. Here, the training dataset is the periodic hills PHLL4 set: (a) true  $g^{(1)}$  field; (b) predicted  $g^{(1)}$  field; (c) true  $g^{(2)}$  field; (d) predicted  $g^{(2)}$  field; (e) true  $g^{(3)}$  field; and, (f) predicted  $g^{(3)}$  field.

### 3.1.3 XGBoost

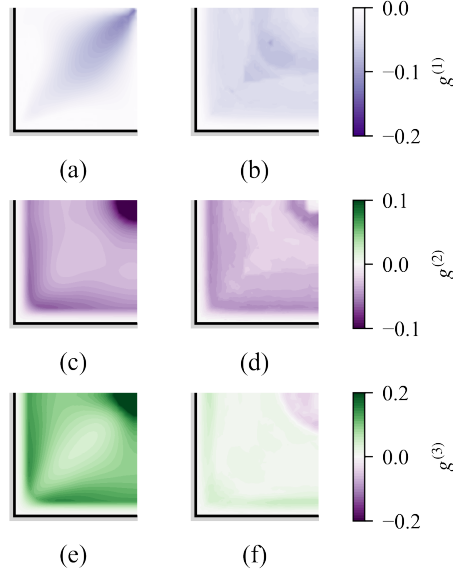

Figure 27: Generalizability test on the square duct test case for the XGBoost model. Here, the training dataset is the periodic hills PHLL4 set: (a) true  $g^{(1)}$  field; (b) predicted  $g^{(1)}$  field; (c) true  $g^{(2)}$  field; (d) predicted  $g^{(2)}$  field; (e) true  $g^{(3)}$  field; and, (f) predicted  $g^{(3)}$  field.

## 3.2 BUMP4 training set

### 3.2.1 Neural network

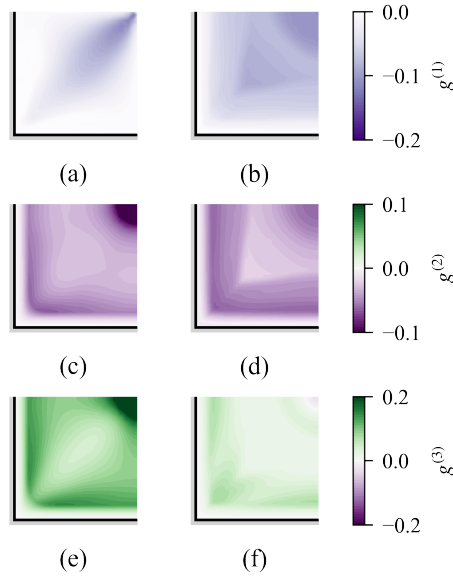

Figure 28: Generalizability test on the square duct test case for the neural network model. Here, the training dataset is the parametric bump BUMP4 set: (a) true  $g^{(1)}$  field; (b) predicted  $g^{(1)}$  field; (c) true  $g^{(2)}$  field; (d) predicted  $g^{(2)}$  field; (e) true  $g^{(3)}$  field; and, (f) predicted  $g^{(3)}$  field.

### 3.2.2 Random forest

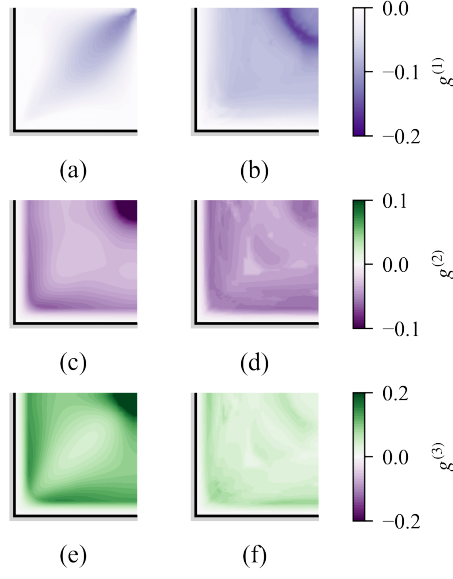

Figure 29: Generalizability test on the square duct test case for the random forest model. Here, the training dataset is the parametric bump BUMP4 set: (a) true  $g^{(1)}$  field; (b) predicted  $g^{(1)}$  field; (c) true  $g^{(2)}$  field; (d) predicted  $g^{(2)}$  field; (e) true  $g^{(3)}$  field; and, (f) predicted  $g^{(3)}$  field.

### 3.2.3 XGBoost

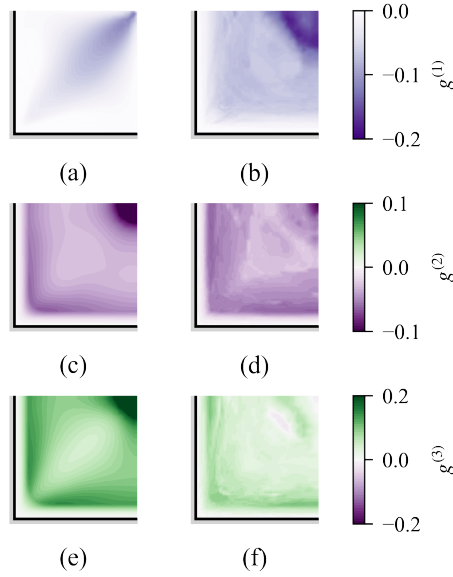

Figure 30: Generalizability test on the square duct test case for the XGBoost model. Here, the training dataset is the parametric bump BUMP4 set: (a) true  $g^{(1)}$  field; (b) predicted  $g^{(1)}$  field; (c) true  $g^{(2)}$  field; (d) predicted  $g^{(2)}$  field; (e) true  $g^{(3)}$  field; and, (f) predicted  $g^{(3)}$  field.

### 3.3 DUCT15 training set

#### 3.3.1 Neural network

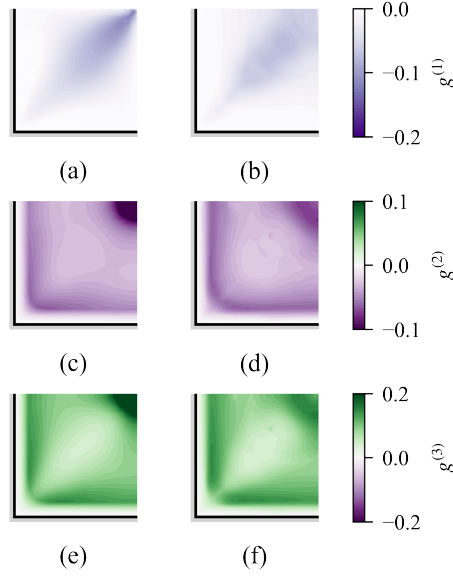

Figure 31: Generalizability test on the square duct test case for the neural network model. Here, the training dataset is the square duct DUCT15 set: (a) true  $g^{(1)}$  field; (b) predicted  $g^{(1)}$  field; (c) true  $g^{(2)}$  field; (d) predicted  $g^{(2)}$  field; (e) true  $g^{(3)}$  field; and, (f) predicted  $g^{(3)}$  field.

#### 3.3.2 Random forest

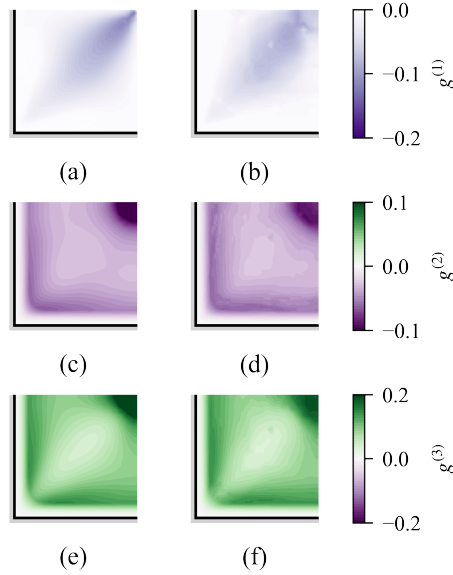

Figure 32: Generalizability test on the square duct test case for the random forest model. Here, the training dataset is the square duct DUCT15 set: (a) true  $g^{(1)}$  field; (b) predicted  $g^{(1)}$  field; (c) true  $g^{(2)}$  field; (d) predicted  $g^{(2)}$  field; (e) true  $g^{(3)}$  field; and, (f) predicted  $g^{(3)}$  field.

### 3.3.3 XGBoost

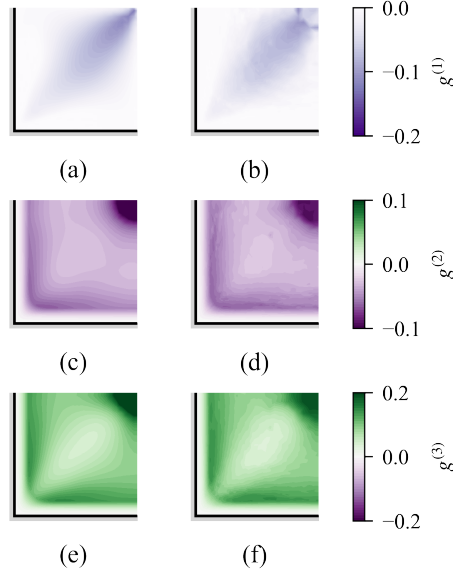

Figure 33: Generalizability test on the square duct test case for the XGBoost model. Here, the training dataset is the square duct DUCT15 set: (a) true  $g^{(1)}$  field; (b) predicted  $g^{(1)}$  field; (c) true  $g^{(2)}$  field; (d) predicted  $g^{(2)}$  field; (e) true  $g^{(3)}$  field; and, (f) predicted  $g^{(3)}$  field.

## 3.4 FULL training set

### 3.4.1 Neural network

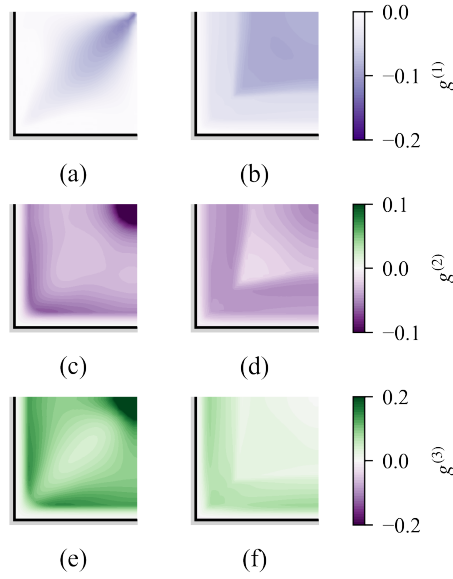

Figure 34: Generalizability test on the square duct test case for the neural network model. Here, the training dataset is the FULL set: (a) true  $g^{(1)}$  field; (b) predicted  $g^{(1)}$  field; (c) true  $g^{(2)}$  field; (d) predicted  $g^{(2)}$  field; (e) true  $g^{(3)}$  field; and, (f) predicted  $g^{(3)}$  field.



### 3.4.2 Random forest

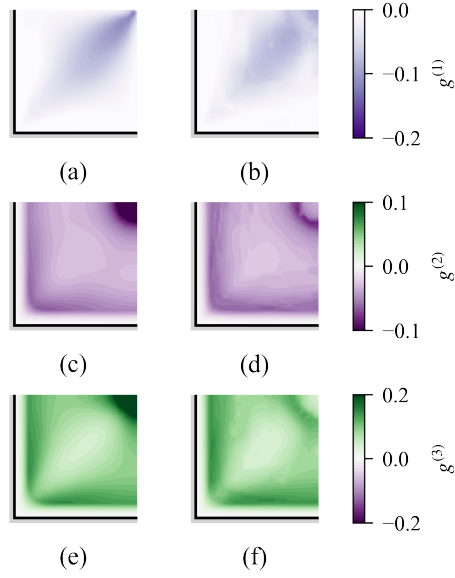

Figure 35: Generalizability test on the square duct test case for the random forest model. Here, the training dataset is the FULL set: (a) true  $g^{(1)}$  field; (b) predicted  $g^{(1)}$  field; (c) true  $g^{(2)}$  field; (d) predicted  $g^{(2)}$  field; (e) true  $g^{(3)}$  field; and, (f) predicted  $g^{(3)}$  field.

### 3.4.3 XGBoost

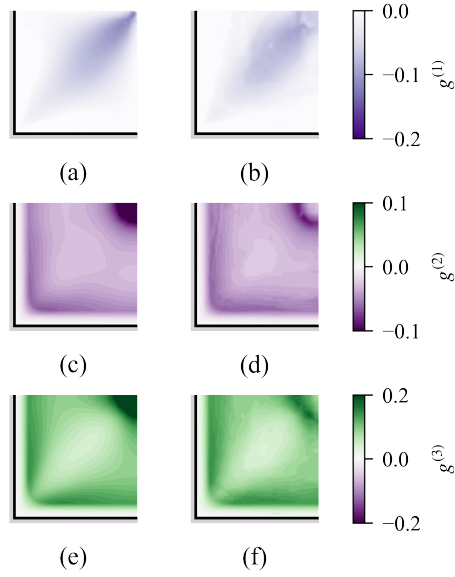

Figure 36: Generalizability test on the square duct test case for the XGBoost model. Here, the training dataset is the FULL set: (a) true  $g^{(1)}$  field; (b) predicted  $g^{(1)}$  field; (c) true  $g^{(2)}$  field; (d) predicted  $g^{(2)}$  field; (e) true  $g^{(3)}$  field; and, (f) predicted  $g^{(3)}$  field.

## 4 Converging-diverging channel test set

### 4.1 PHLL4 training set

#### 4.1.1 Neural network

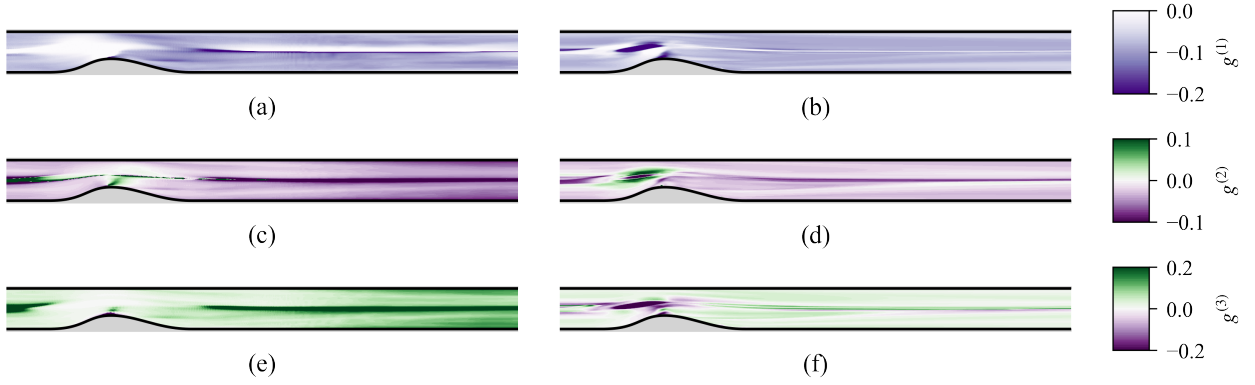

Figure 37: Generalizability test on the converging-diverging channel test case for the neural network model. Here, the training dataset is the periodic hills PHLL4 set: (a) true  $g^{(1)}$  field; (b) predicted  $g^{(1)}$  field; (c) true  $g^{(2)}$  field; (d) predicted  $g^{(2)}$  field; (e) true  $g^{(3)}$  field; and, (f) predicted  $g^{(3)}$  field.

#### 4.1.2 Random forest

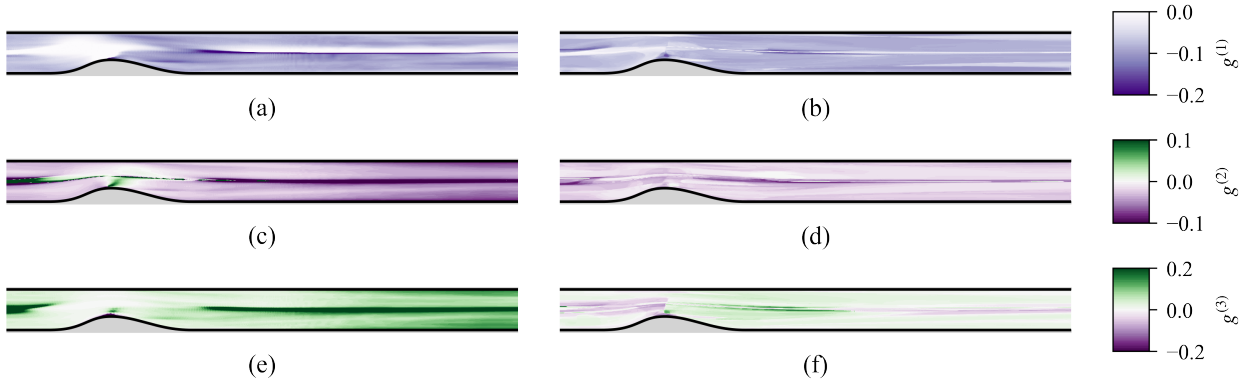

Figure 38: Generalizability test on the converging-diverging channel test case for the random forest model. Here, the training dataset is the periodic hills PHLL4 set: (a) true  $g^{(1)}$  field; (b) predicted  $g^{(1)}$  field; (c) true  $g^{(2)}$  field; (d) predicted  $g^{(2)}$  field; (e) true  $g^{(3)}$  field; and, (f) predicted  $g^{(3)}$  field.

### 4.1.3 XGBoost

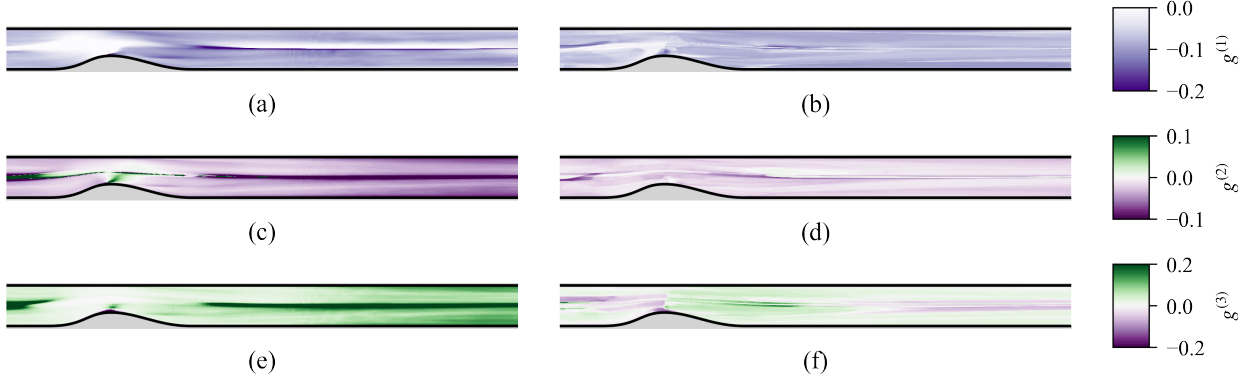

Figure 39: Generalizability test on the converging-diverging channel test case for the XGBoost model. Here, the training dataset is the periodic hills PHLL4 set: (a) true  $g^{(1)}$  field; (b) predicted  $g^{(1)}$  field; (c) true  $g^{(2)}$  field; (d) predicted  $g^{(2)}$  field; (e) true  $g^{(3)}$  field; and, (f) predicted  $g^{(3)}$  field.

## 4.2 BUMP4 training set

### 4.2.1 Neural network

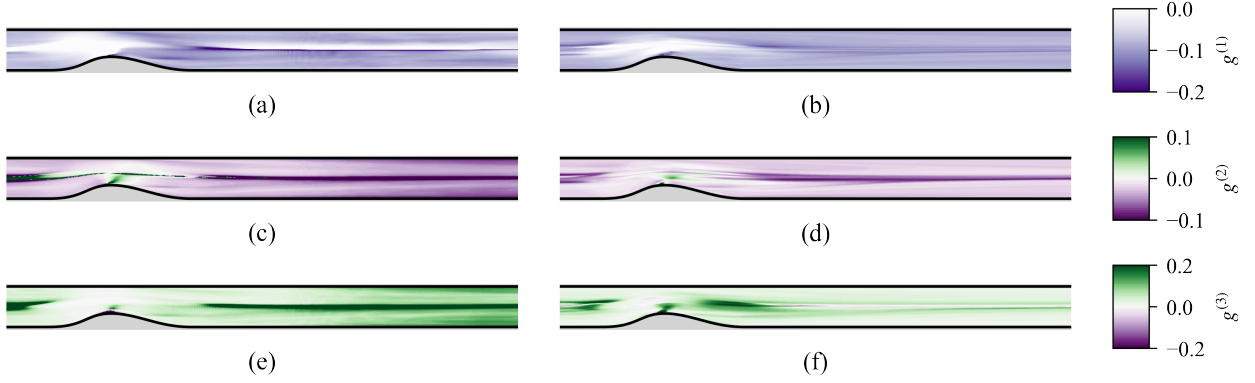

Figure 40: Generalizability test on the converging-diverging channel test case for the neural network model. Here, the training dataset is the parametric bump BUMP4 set: (a) true  $g^{(1)}$  field; (b) predicted  $g^{(1)}$  field; (c) true  $g^{(2)}$  field; (d) predicted  $g^{(2)}$  field; (e) true  $g^{(3)}$  field; and, (f) predicted  $g^{(3)}$  field.

### 4.2.2 Random forest

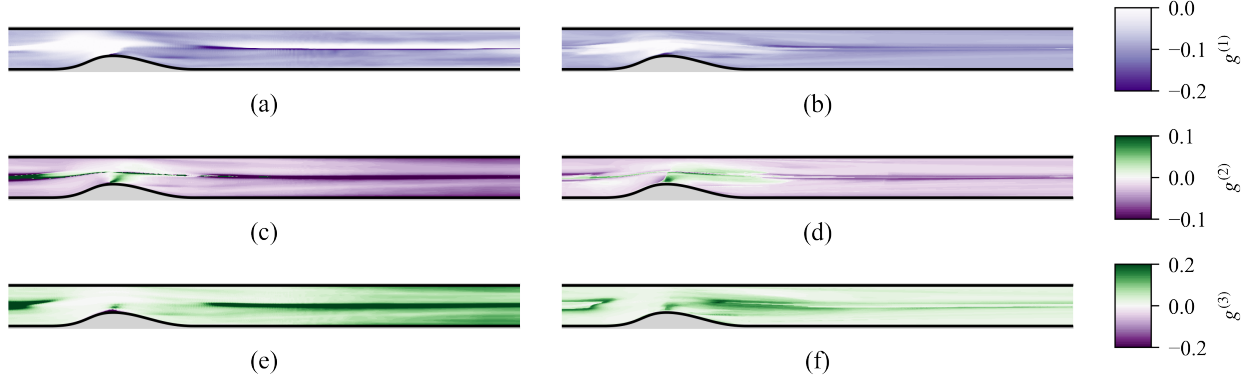

Figure 41: Generalizability test on the converging-diverging channel test case for the random forest model. Here, the training dataset is the parametric bump BUMP4 set: (a) true  $g^{(1)}$  field; (b) predicted  $g^{(1)}$  field; (c) true  $g^{(2)}$  field; (d) predicted  $g^{(2)}$  field; (e) true  $g^{(3)}$  field; and, (f) predicted  $g^{(3)}$  field.

### 4.2.3 XGBoost

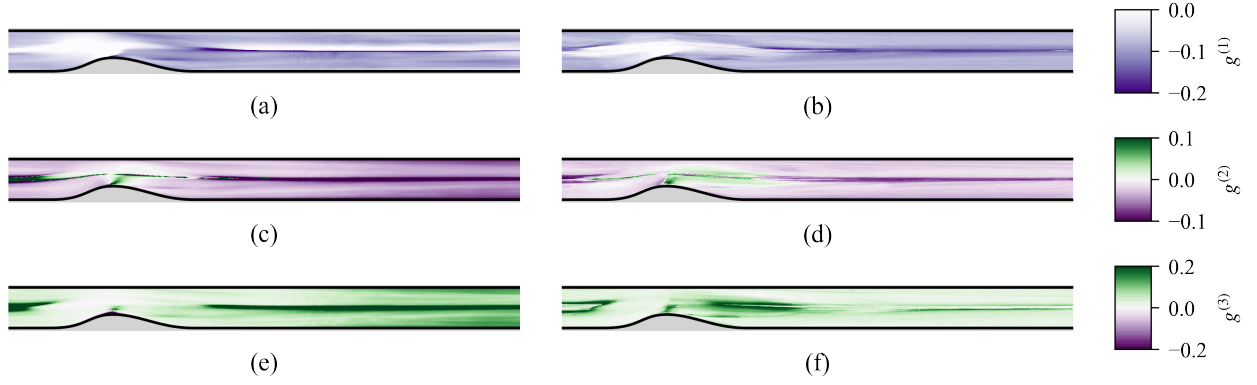

Figure 42: Generalizability test on the converging-diverging channel test case for the XGBoost model. Here, the training dataset is the parametric bump BUMP4 set: (a) true  $g^{(1)}$  field; (b) predicted  $g^{(1)}$  field; (c) true  $g^{(2)}$  field; (d) predicted  $g^{(2)}$  field; (e) true  $g^{(3)}$  field; and, (f) predicted  $g^{(3)}$  field.

### 4.3 DUCT15 training set

#### 4.3.1 Neural network

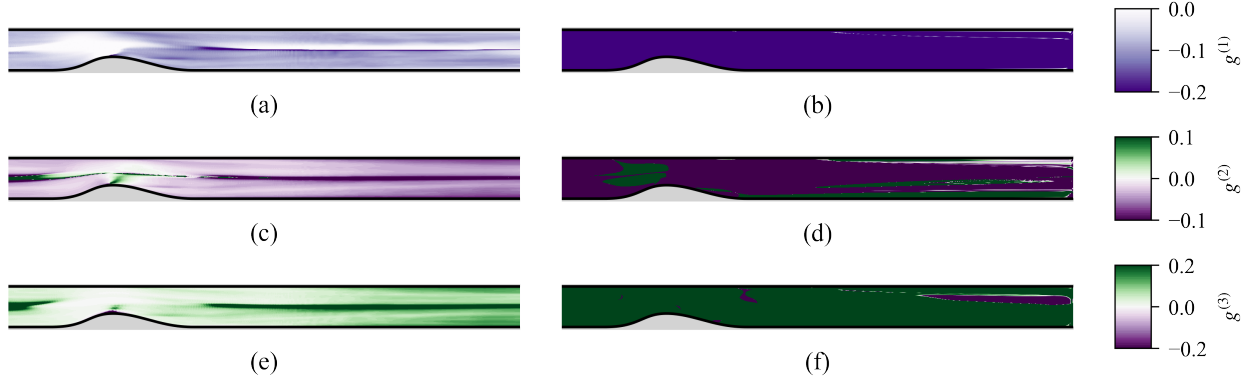

Figure 43: Generalizability test on the converging-diverging channel test case for the neural network model. Here, the training dataset is the square duct DUCT15 set: (a) true  $g^{(1)}$  field; (b) predicted  $g^{(1)}$  field; (c) true  $g^{(2)}$  field; (d) predicted  $g^{(2)}$  field; (e) true  $g^{(3)}$  field; and, (f) predicted  $g^{(3)}$  field.

#### 4.3.2 Random forest

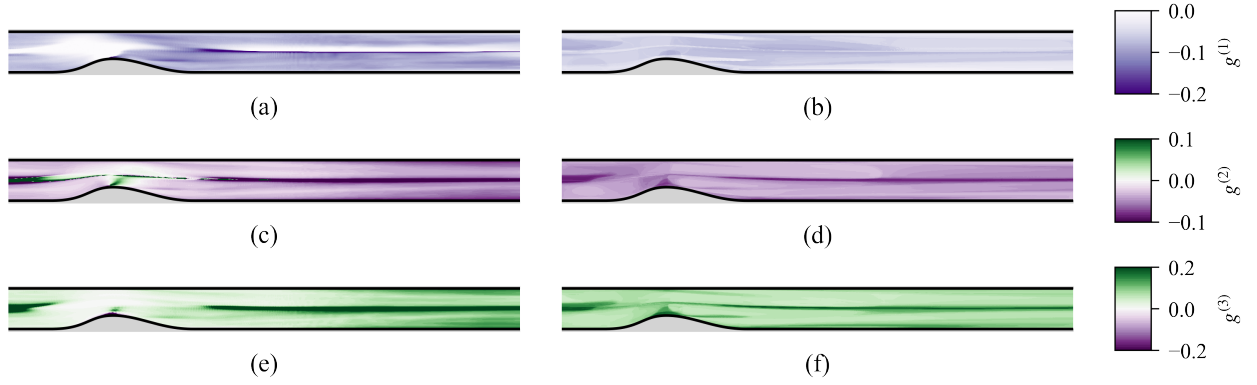

Figure 44: Generalizability test on the converging-diverging channel test case for the random forest model. Here, the training dataset is the square duct DUCT15 set: (a) true  $g^{(1)}$  field; (b) predicted  $g^{(1)}$  field; (c) true  $g^{(2)}$  field; (d) predicted  $g^{(2)}$  field; (e) true  $g^{(3)}$  field; and, (f) predicted  $g^{(3)}$  field.

### 4.3.3 XGBoost

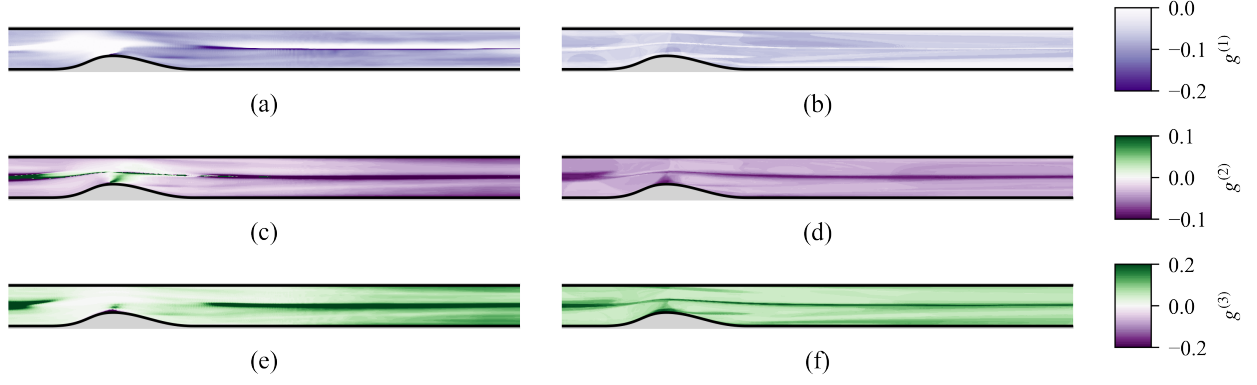

Figure 45: Generalizability test on the converging-diverging channel test case for the XGBoost model. Here, the training dataset is the square duct DUCT15 set: (a) true  $g^{(1)}$  field; (b) predicted  $g^{(1)}$  field; (c) true  $g^{(2)}$  field; (d) predicted  $g^{(2)}$  field; (e) true  $g^{(3)}$  field; and, (f) predicted  $g^{(3)}$  field.

## 4.4 FULL training set

### 4.4.1 Neural network

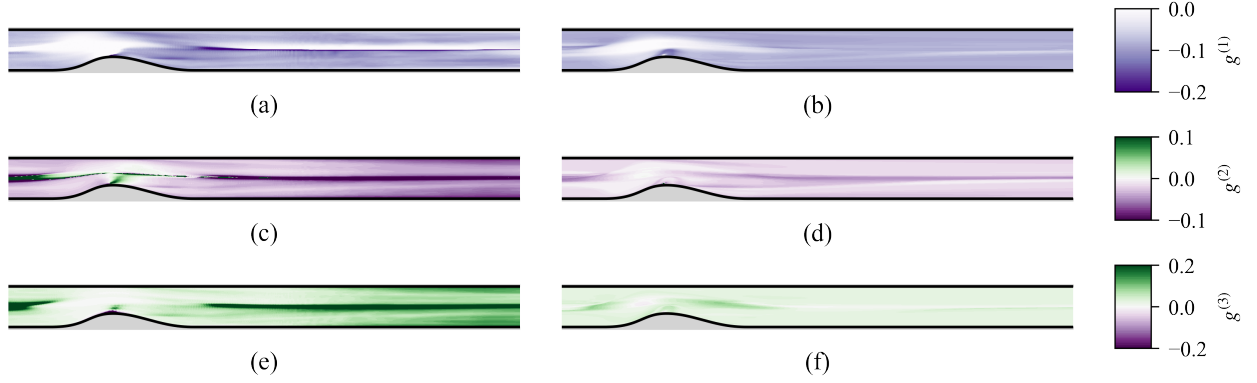

Figure 46: Generalizability test on the converging-diverging channel test case for the neural network model. Here, the training dataset is the FULL set: (a) true  $g^{(1)}$  field; (b) predicted  $g^{(1)}$  field; (c) true  $g^{(2)}$  field; (d) predicted  $g^{(2)}$  field; (e) true  $g^{(3)}$  field; and, (f) predicted  $g^{(3)}$  field.

#### 4.4.2 Random forest

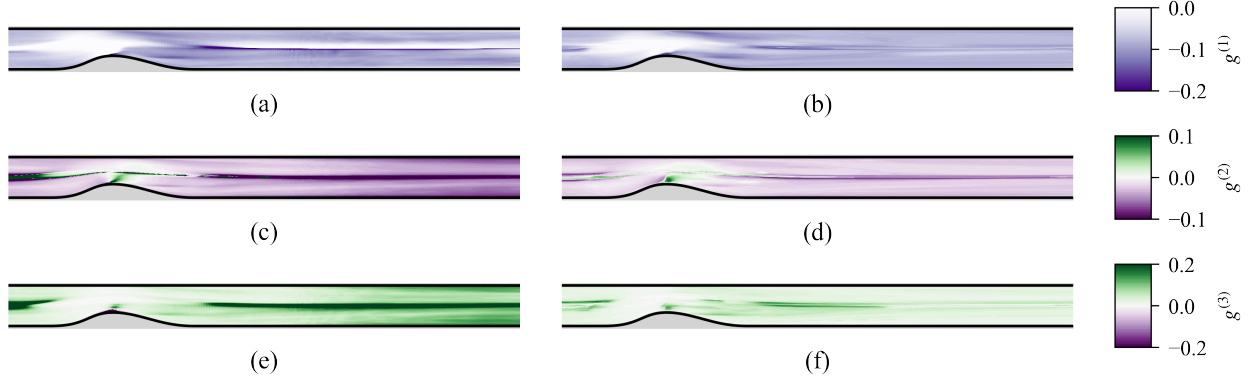

Figure 47: Generalizability test on the converging-diverging channel test case for the random forest model. Here, the training dataset is the FULL set: (a) true  $g^{(1)}$  field; (b) predicted  $g^{(1)}$  field; (c) true  $g^{(2)}$  field; (d) predicted  $g^{(2)}$  field; (e) true  $g^{(3)}$  field; and, (f) predicted  $g^{(3)}$  field.

#### 4.4.3 XGBoost

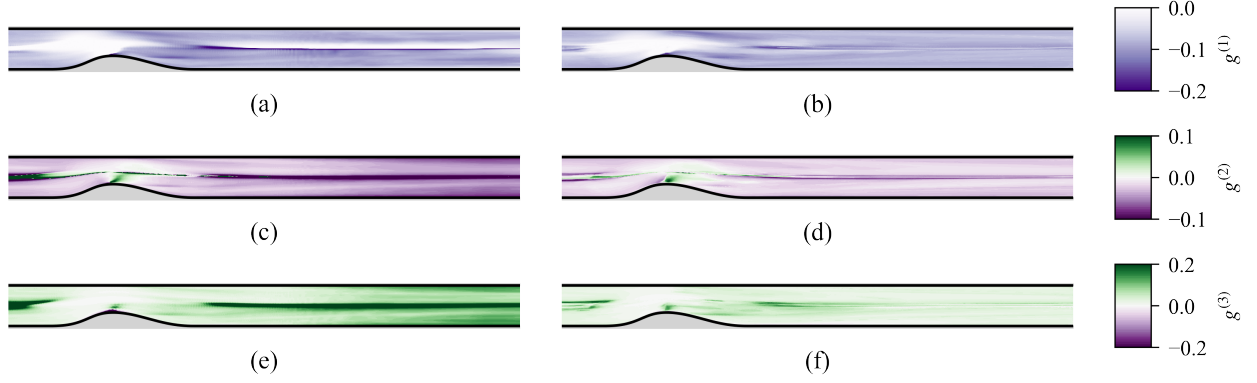

Figure 48: Generalizability test on the converging-diverging channel test case for the XGBoost model. Here, the training dataset is the FULL set: (a) true  $g^{(1)}$  field; (b) predicted  $g^{(1)}$  field; (c) true  $g^{(2)}$  field; (d) predicted  $g^{(2)}$  field; (e) true  $g^{(3)}$  field; and, (f) predicted  $g^{(3)}$  field.

## 5 Curved backward-facing step test set

### 5.1 PHLL4 training set

#### 5.1.1 Neural network

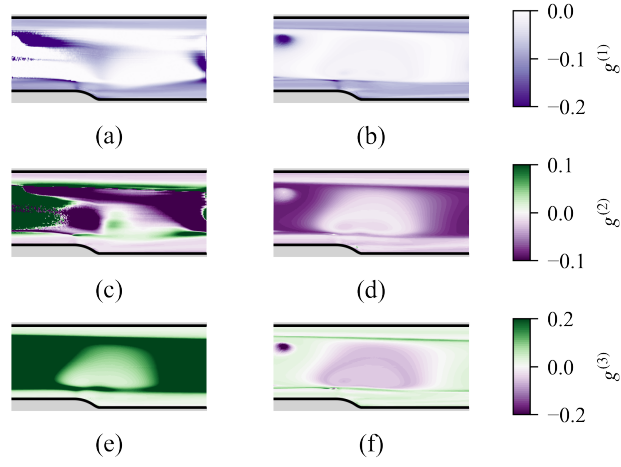

Figure 49: Generalizability test on the curved backward-facing step test case for the neural network model. Here, the training dataset is the periodic hills PHLL4 set: (a) true  $g^{(1)}$  field; (b) predicted  $g^{(1)}$  field; (c) true  $g^{(2)}$  field; (d) predicted  $g^{(2)}$  field; (e) true  $g^{(3)}$  field; and, (f) predicted  $g^{(3)}$  field.

#### 5.1.2 Random forest

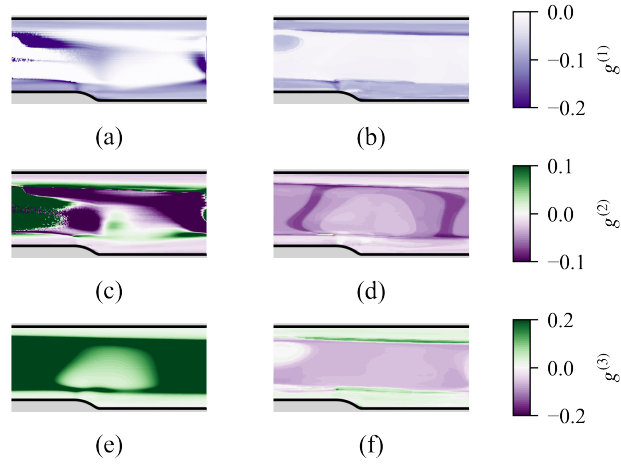

Figure 50: Generalizability test on the curved backward-facing step test case for the random forest model. Here, the training dataset is the periodic hills PHLL4 set: (a) true  $g^{(1)}$  field; (b) predicted  $g^{(1)}$  field; (c) true  $g^{(2)}$  field; (d) predicted  $g^{(2)}$  field; (e) true  $g^{(3)}$  field; and, (f) predicted  $g^{(3)}$  field.



### 5.1.3 XGBoost

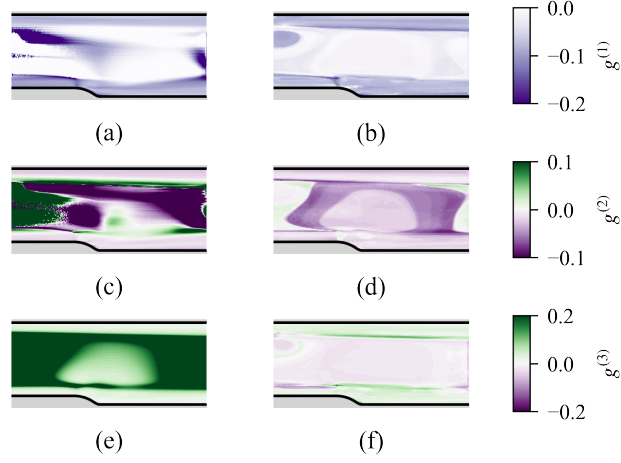

Figure 51: Generalizability test on the curved backward-facing step test case for the XGBoost model. Here, the training dataset is the periodic hills PHLL4 set: (a) true  $g^{(1)}$  field; (b) predicted  $g^{(1)}$  field; (c) true  $g^{(2)}$  field; (d) predicted  $g^{(2)}$  field; (e) true  $g^{(3)}$  field; and, (f) predicted  $g^{(3)}$  field.

## 5.2 BUMP4 training set

### 5.2.1 Neural network

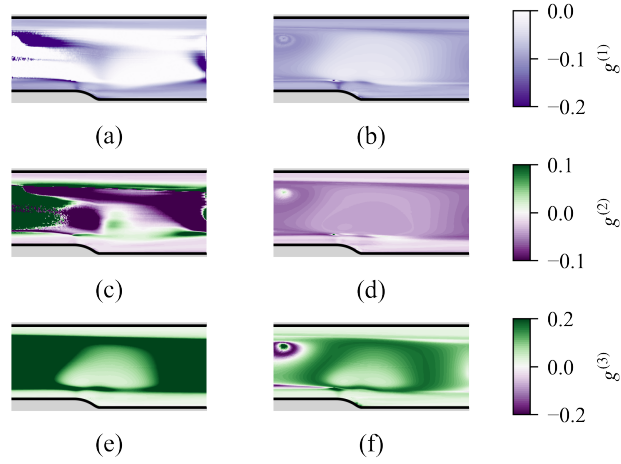

Figure 52: Generalizability test on the curved backward-facing step test case for the neural network model. Here, the training dataset is the parametric bump BUMP4 set: (a) true  $g^{(1)}$  field; (b) predicted  $g^{(1)}$  field; (c) true  $g^{(2)}$  field; (d) predicted  $g^{(2)}$  field; (e) true  $g^{(3)}$  field; and, (f) predicted  $g^{(3)}$  field.

### 5.2.2 Random forest

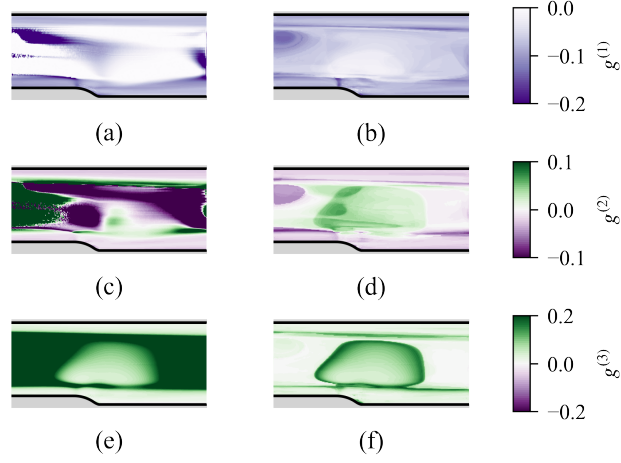

Figure 53: Generalizability test on the curved backward-facing step test case for the random forest model. Here, the training dataset is the parametric bump BUMP4 set: (a) true  $g^{(1)}$  field; (b) predicted  $g^{(1)}$  field; (c) true  $g^{(2)}$  field; (d) predicted  $g^{(2)}$  field; (e) true  $g^{(3)}$  field; and, (f) predicted  $g^{(3)}$  field.

### 5.2.3 XGBoost

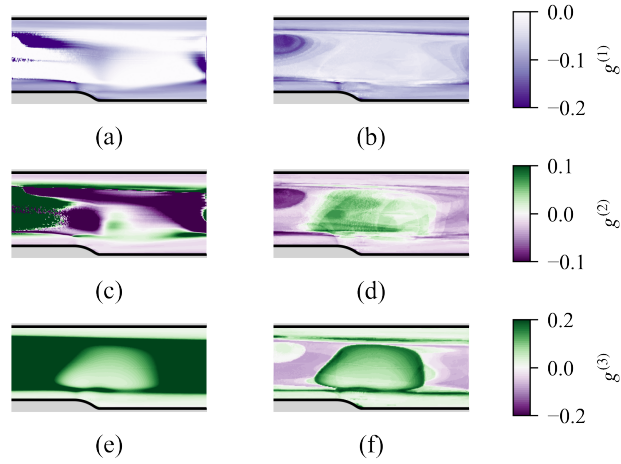

Figure 54: Generalizability test on the curved backward-facing step test case for the XGBoost model. Here, the training dataset is the parametric bump BUMP4 set: (a) true  $g^{(1)}$  field; (b) predicted  $g^{(1)}$  field; (c) true  $g^{(2)}$  field; (d) predicted  $g^{(2)}$  field; (e) true  $g^{(3)}$  field; and, (f) predicted  $g^{(3)}$  field.

### 5.3 DUCT15 training set

#### 5.3.1 Neural network

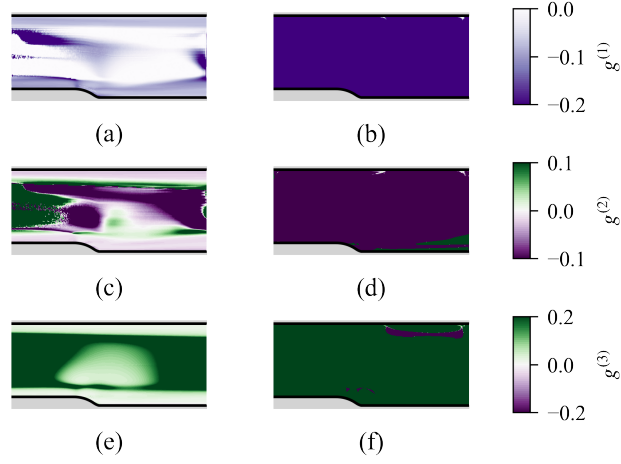

Figure 55: Generalizability test on the curved backward-facing step test case for the neural network model. Here, the training dataset is the square duct DUCT15 set: (a) true  $g^{(1)}$  field; (b) predicted  $g^{(1)}$  field; (c) true  $g^{(2)}$  field; (d) predicted  $g^{(2)}$  field; (e) true  $g^{(3)}$  field; and, (f) predicted  $g^{(3)}$  field.

#### 5.3.2 Random forest

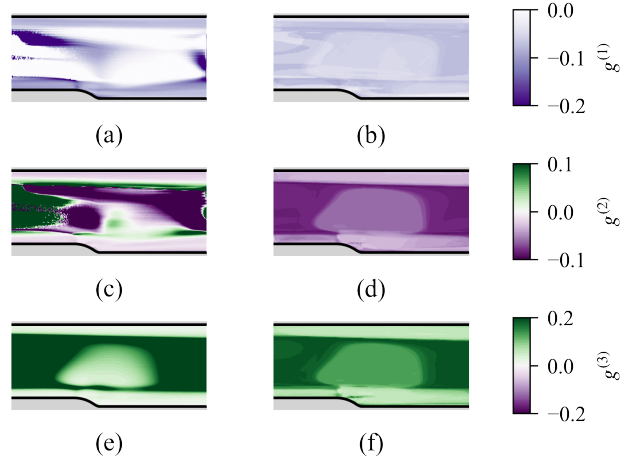

Figure 56: Generalizability test on the curved backward-facing step test case for the random forest model. Here, the training dataset is the square duct DUCT15 set: (a) true  $g^{(1)}$  field; (b) predicted  $g^{(1)}$  field; (c) true  $g^{(2)}$  field; (d) predicted  $g^{(2)}$  field; (e) true  $g^{(3)}$  field; and, (f) predicted  $g^{(3)}$  field.

### 5.3.3 XGBoost

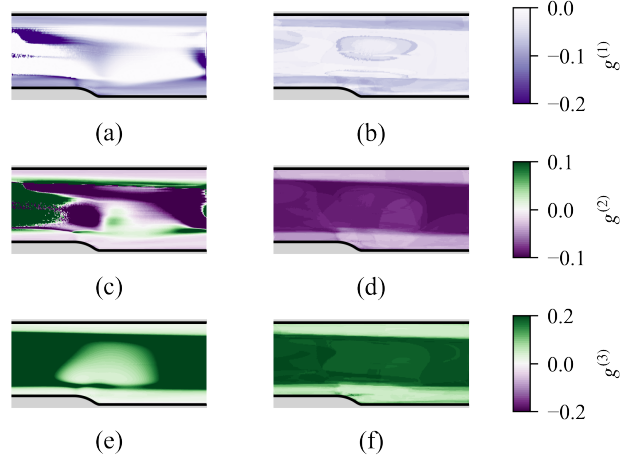

Figure 57: Generalizability test on the curved backward-facing step test case for the XGBoost model. Here, the training dataset is the square duct DUCT15 set: (a) true  $g^{(1)}$  field; (b) predicted  $g^{(1)}$  field; (c) true  $g^{(2)}$  field; (d) predicted  $g^{(2)}$  field; (e) true  $g^{(3)}$  field; and, (f) predicted  $g^{(3)}$  field.

## 5.4 FULL training set

### 5.4.1 Neural network

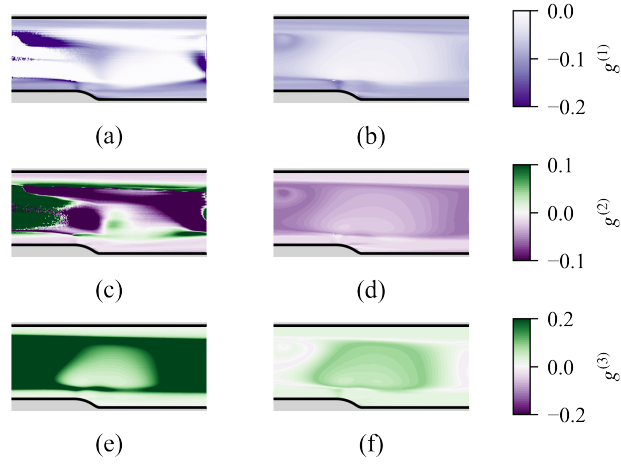

Figure 58: Generalizability test on the curved backward-facing step test case for the neural network model. Here, the training dataset is the FULL set: (a) true  $g^{(1)}$  field; (b) predicted  $g^{(1)}$  field; (c) true  $g^{(2)}$  field; (d) predicted  $g^{(2)}$  field; (e) true  $g^{(3)}$  field; and, (f) predicted  $g^{(3)}$  field.

### 5.4.2 Random forest

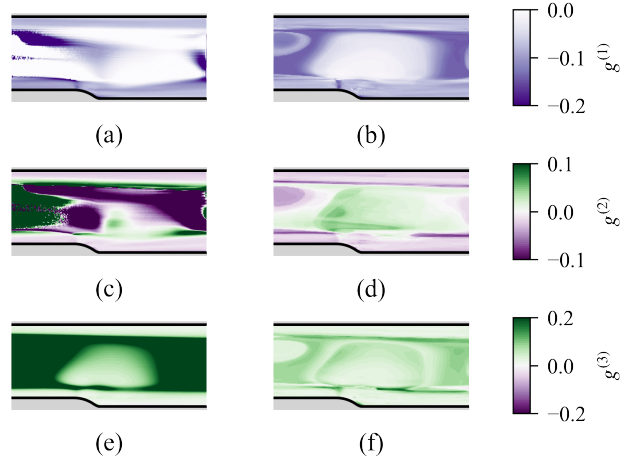

Figure 59: Generalizability test on the curved backward-facing step test case for the random forest model. Here, the training dataset is the FULL set: (a) true  $g^{(1)}$  field; (b) predicted  $g^{(1)}$  field; (c) true  $g^{(2)}$  field; (d) predicted  $g^{(2)}$  field; (e) true  $g^{(3)}$  field; and, (f) predicted  $g^{(3)}$  field.

### 5.4.3 XGBoost

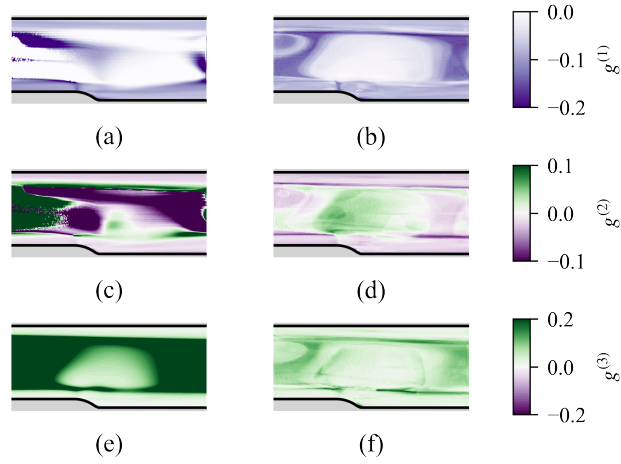

Figure 60: Generalizability test on the curved backward-facing step test case for the XGBoost model. Here, the training dataset is the FULL set: (a) true  $g^{(1)}$  field; (b) predicted  $g^{(1)}$  field; (c) true  $g^{(2)}$  field; (d) predicted  $g^{(2)}$  field; (e) true  $g^{(3)}$  field; and, (f) predicted  $g^{(3)}$  field.
